# Supplementary material for: Aquarium: A Comprehensive Framework for Exploring Predator-Prey Dynamics through Multi-Agent Reinforcement Learning Algorithms
Source: arXiv:2401.07056 source file (2024-01-13)
Supplement: Supplementary file 1 [file X_appendix.tex]

\begin{table*}[t]
\begin{center}
\adjustbox{width=0.8\linewidth}{
\begin{tabular}{lccl}
\hline
Parameter & Data Type & Default Value & Explanation \\
\hline

Width & Integer & 800 & Width of the environment \\
Height & Integer & 800 & Height of the environment \\
FPS & Integer & 60 & Frames per second on visualization\\
Max timesteps & Integer & 3000 & Number of timesteps per episode \\
Actions number & Integer & 8 &  Number of available directions for actions\\
Replication & Boolean & False & Prey reproduction\\
FOV enabled & Boolean & False & FOV for agent's vision\\
Draw action Vectors & Boolean & True & Draw the Vector visualizing the agents action\\
Draw hit box & Boolean & False & Draw hitbox around agents\\
Draw capture points & Boolean & False & Draw red points where prey agents were captures\\
Constant fish number & Boolean & True & Respawn fish after being caught or not\\
Record & Boolean & False & Saving of episode as video file\\
Max steer force & Float & 0.6 & Steering force magnitude multiplier\\

Shark number & Integer & 1 & Number of sharks\\
Shark max acceleration & Float & 0.6 & Maximum acceleration of a shark\\
Shark radius & Integer & 30 & Hitbox radius of shark\\
Shark max velocity & Integer & 5 & Maximum velocity of shark\\
Shark view distance & Integer & 200 & Distance shark can see\\
Observed fish number & Integer & 8 & Number of fish that a learning shark is capable of perceiving\\
Shark starvation age & Integer & 3000 & Number of time steps without captures until sharks starves\\
Shark view angle & Integer & 150 & View angle of shark\\

Fish number & Integer & 8 & Initial number of fish\\
Fish max acceleration & Float & 1 & Maximum acceleration of fish\\
Fish radius & Integer & 20 & Hitbox radius of fish\\
Fish max velocity & Integer & 4 & Maximum velocity of fish\\
Fish view distance & Integer & 100 & Distance fish can see\\
Fish replication age & Integer & 200 & Number of time steps after which a fish can be replicated\\
Fish view angle & Integer & 100 & View angle of fish\\
Max fish number & Integer & 20 & Maximum number of fish \\
\hline
\end{tabular}
}
\end{center}

\caption{This table shows all available adjustable parameters of the Aquarium environment, along with their data types, default values, and explanations}
\label{tab:config}
\end{table*}

\section*{\uppercase{Appendix}}

\subsection*{Environment Customization}\label{sec:debugging}

The Aquarium environment allows the manipulation and creation of diverse configurations and visual styles. Numerous of the accessible parameters have been introduced in the preceding sections. A complete summary of all available parameters, along with their respective data types, default values, and explanations is provided in \Cref{tab:config}. This allows for straightforward experimentation with various predator-prey configurations.

The visual representation of predator and prey can be easily customized to accommodate diverse predator-prey scenarios. Additionally, Aquarium allows the visualization of various agent attributes. The agent's FOV can be visualized in different colors for both types of agents. Moreover, an agent's action vector designated by its policy, its current velocity, and its current acceleration vector can be incorporated into the visualization for each individual agent. In addition, it is possible to highlight the location where a prey has been captured by a predator. Furthermore, the integration of the PettingZoo library enhances the environment by offering the capability to record the rendering of the environment. This addition brings the advantage of preserving and analyzing the visual representation of the dynamic scenarios that unfold during agent training and evaluation. \Cref{fig:visualization_examples} illustrates some instances of these attribute visualizations.

\begin{figure}[htb]
    \centering
    \includegraphics[width=\columnwidth]{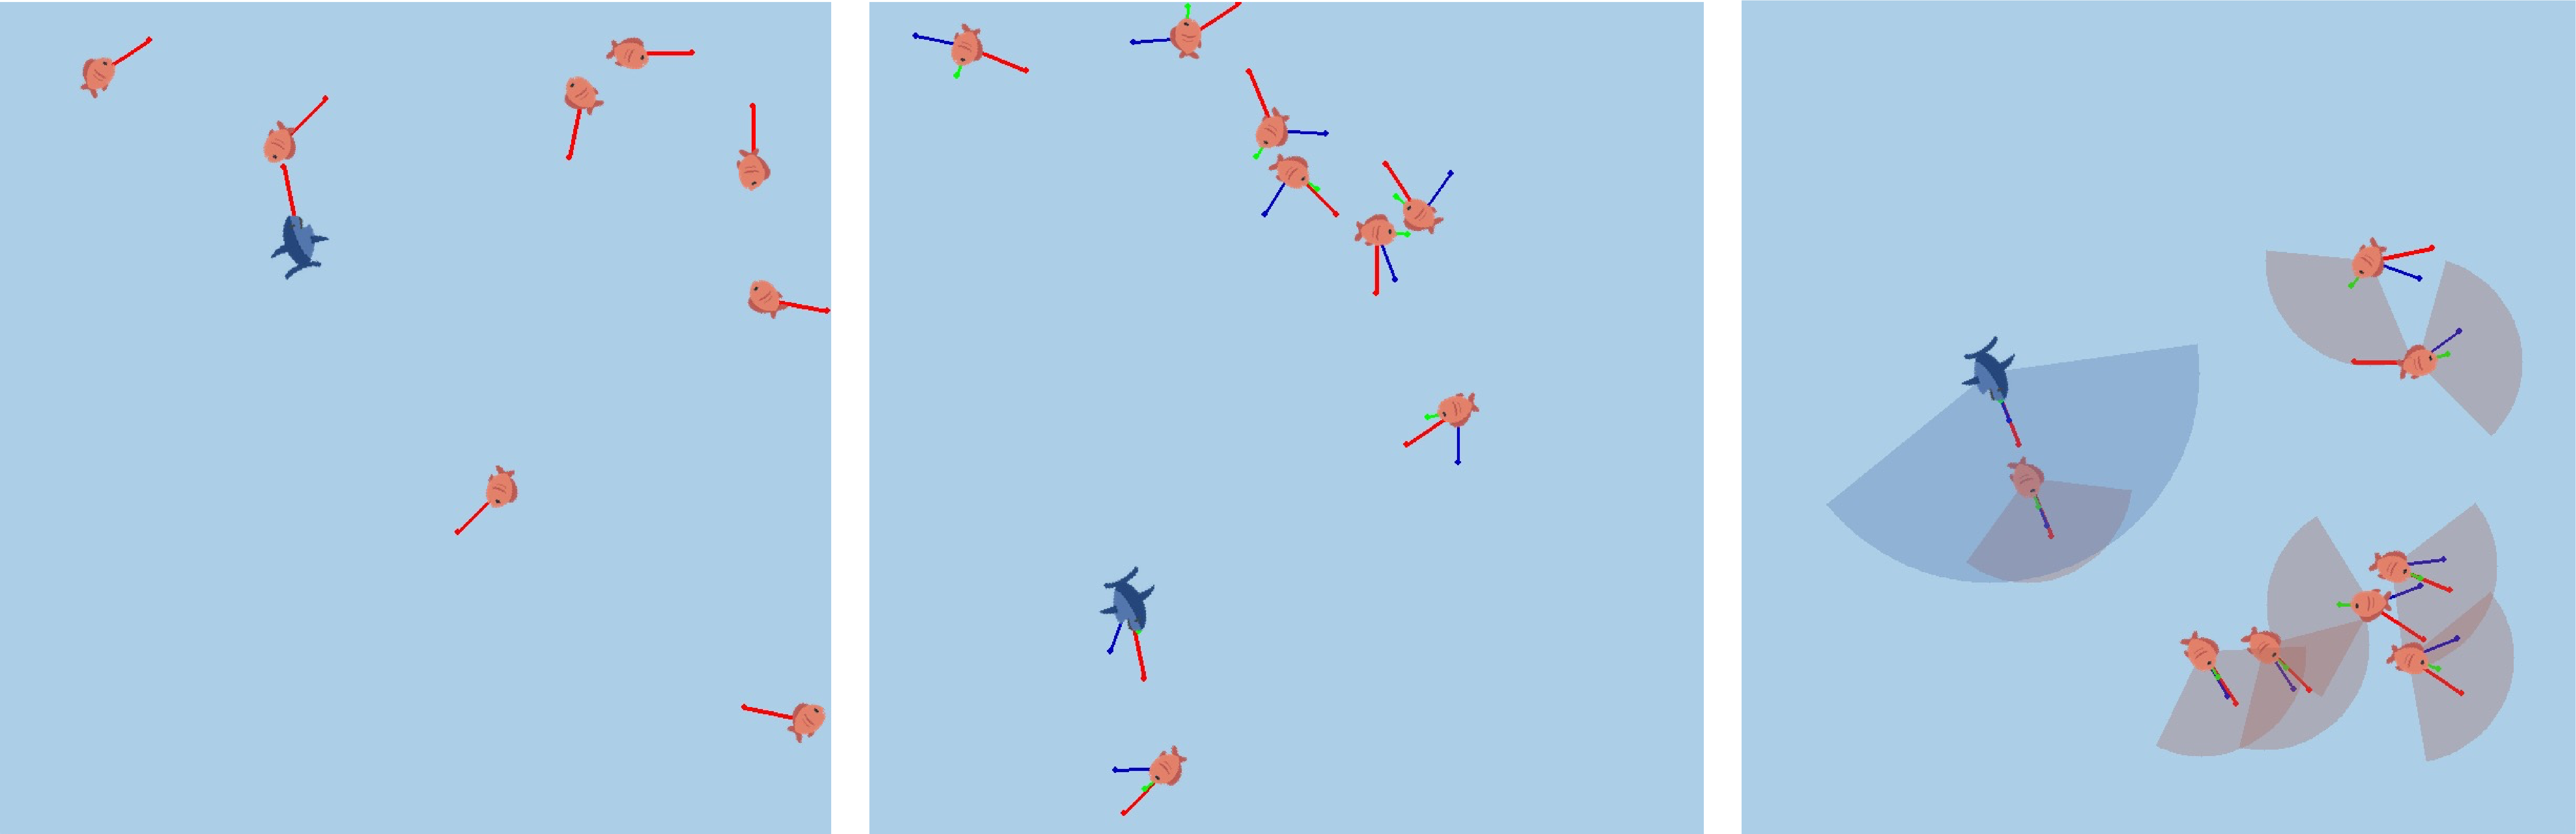}
    \caption{The environment depicts various attributes: an agent's policy-directed action vector in red (left), current velocity and acceleration in blue and green, respectively (middle), and distinct agent types' FOV in varied colors (right).}
    \label{fig:visualization_examples}
\end{figure}

% \begin{figure}[htbp]
%     \centering
%     \includegraphics[width=\columnwidth]{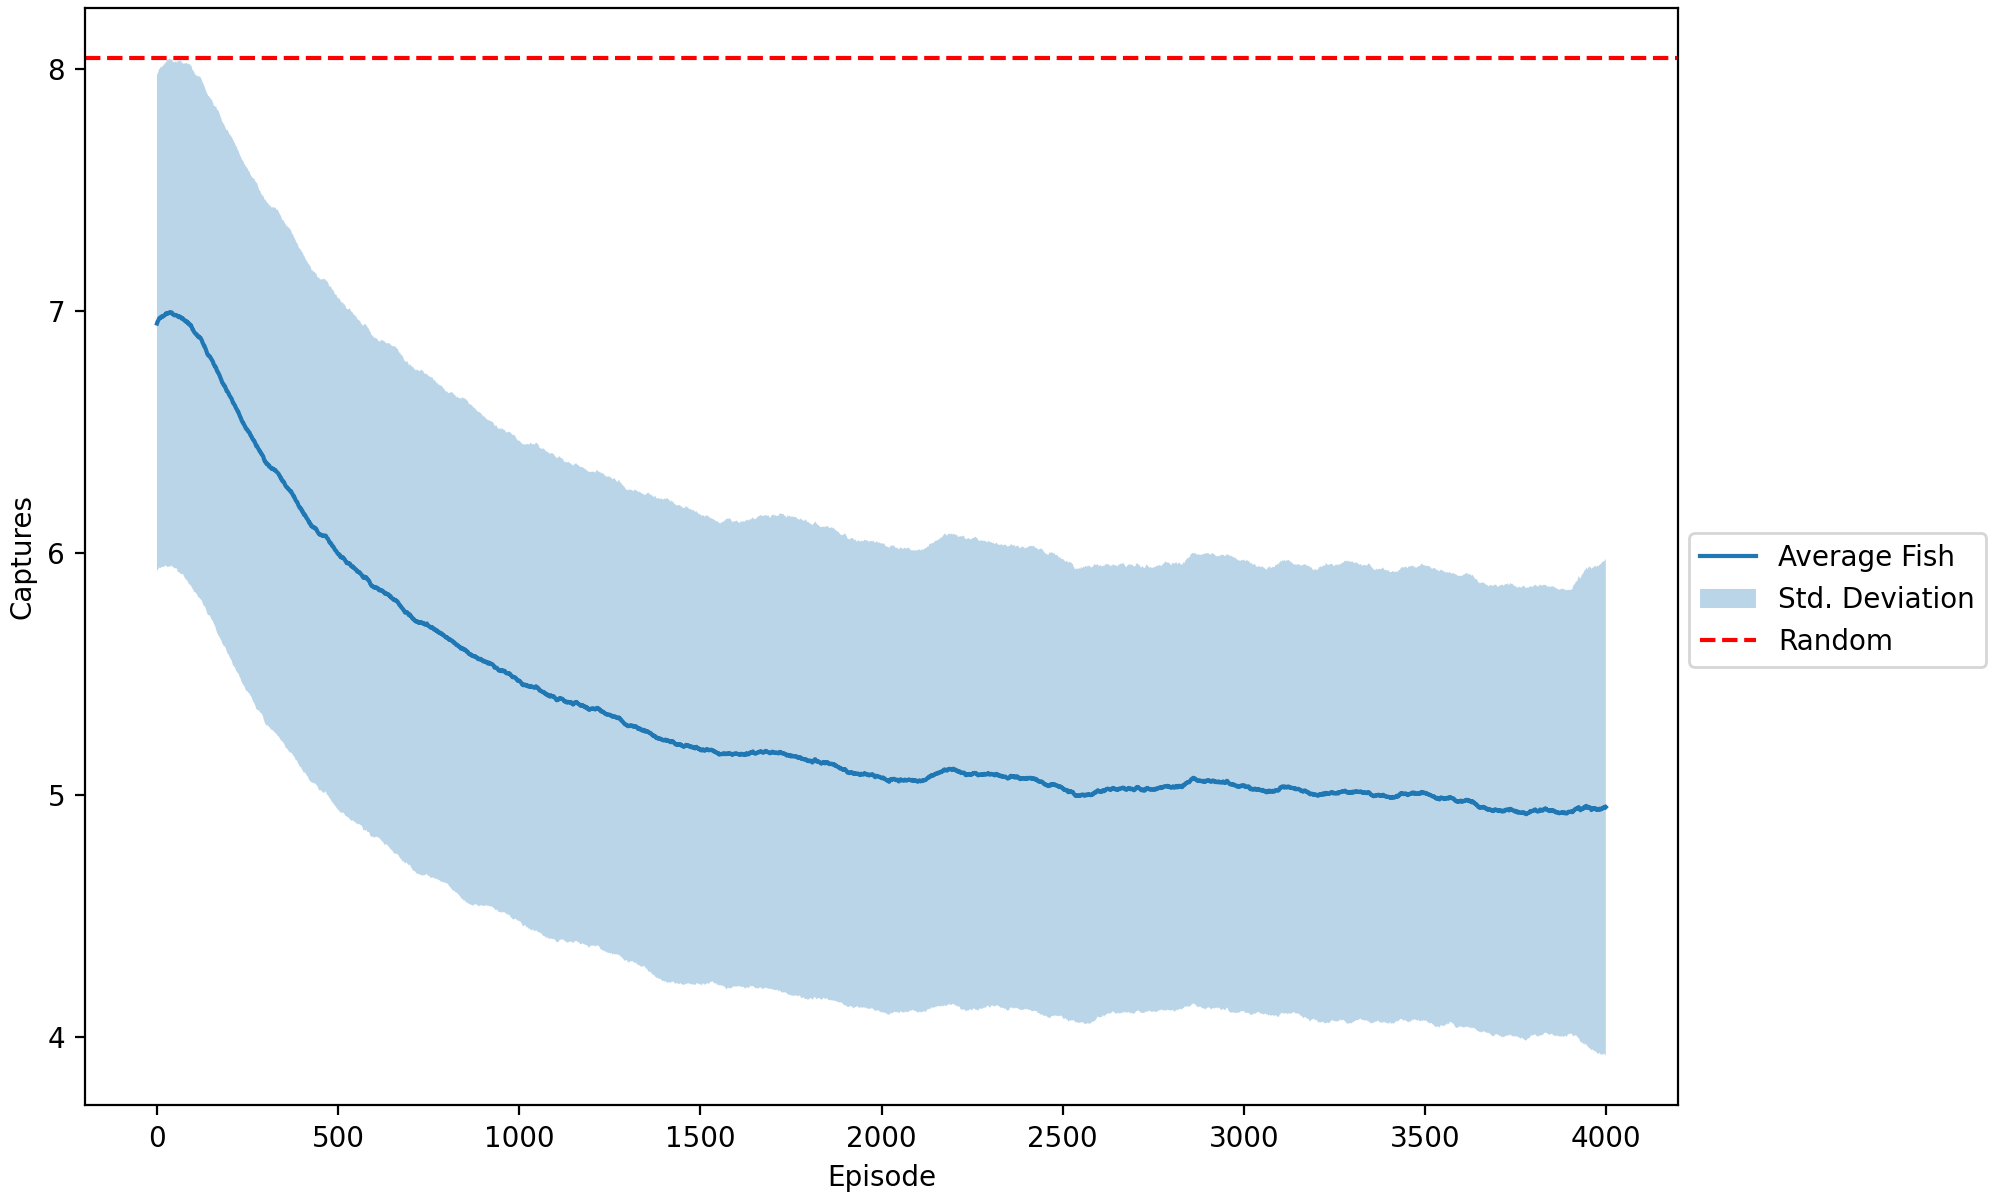}
%     \caption[Average Captures per Prey Agent Using the Individual Training Strategy.]{Average Captures per Prey Agent Using the Individual Training Strategy. Training was performed for 6000 episodes, each lasting $3000$ time steps. The prey agents were individually trained, such that each agent is equipped with its unique policy and exclusively learns from its own experiences. The individual captures over the six prey agents were averaged for each episode and the standard deviation was calculated. The red dotted line represents the average capture achieved over all episodes with random behavior.}
%     \label{fig:indi_captures}
% \end{figure}

% \begin{figure}[htbp]
%     \centering
%     \includegraphics[width=\columnwidth]{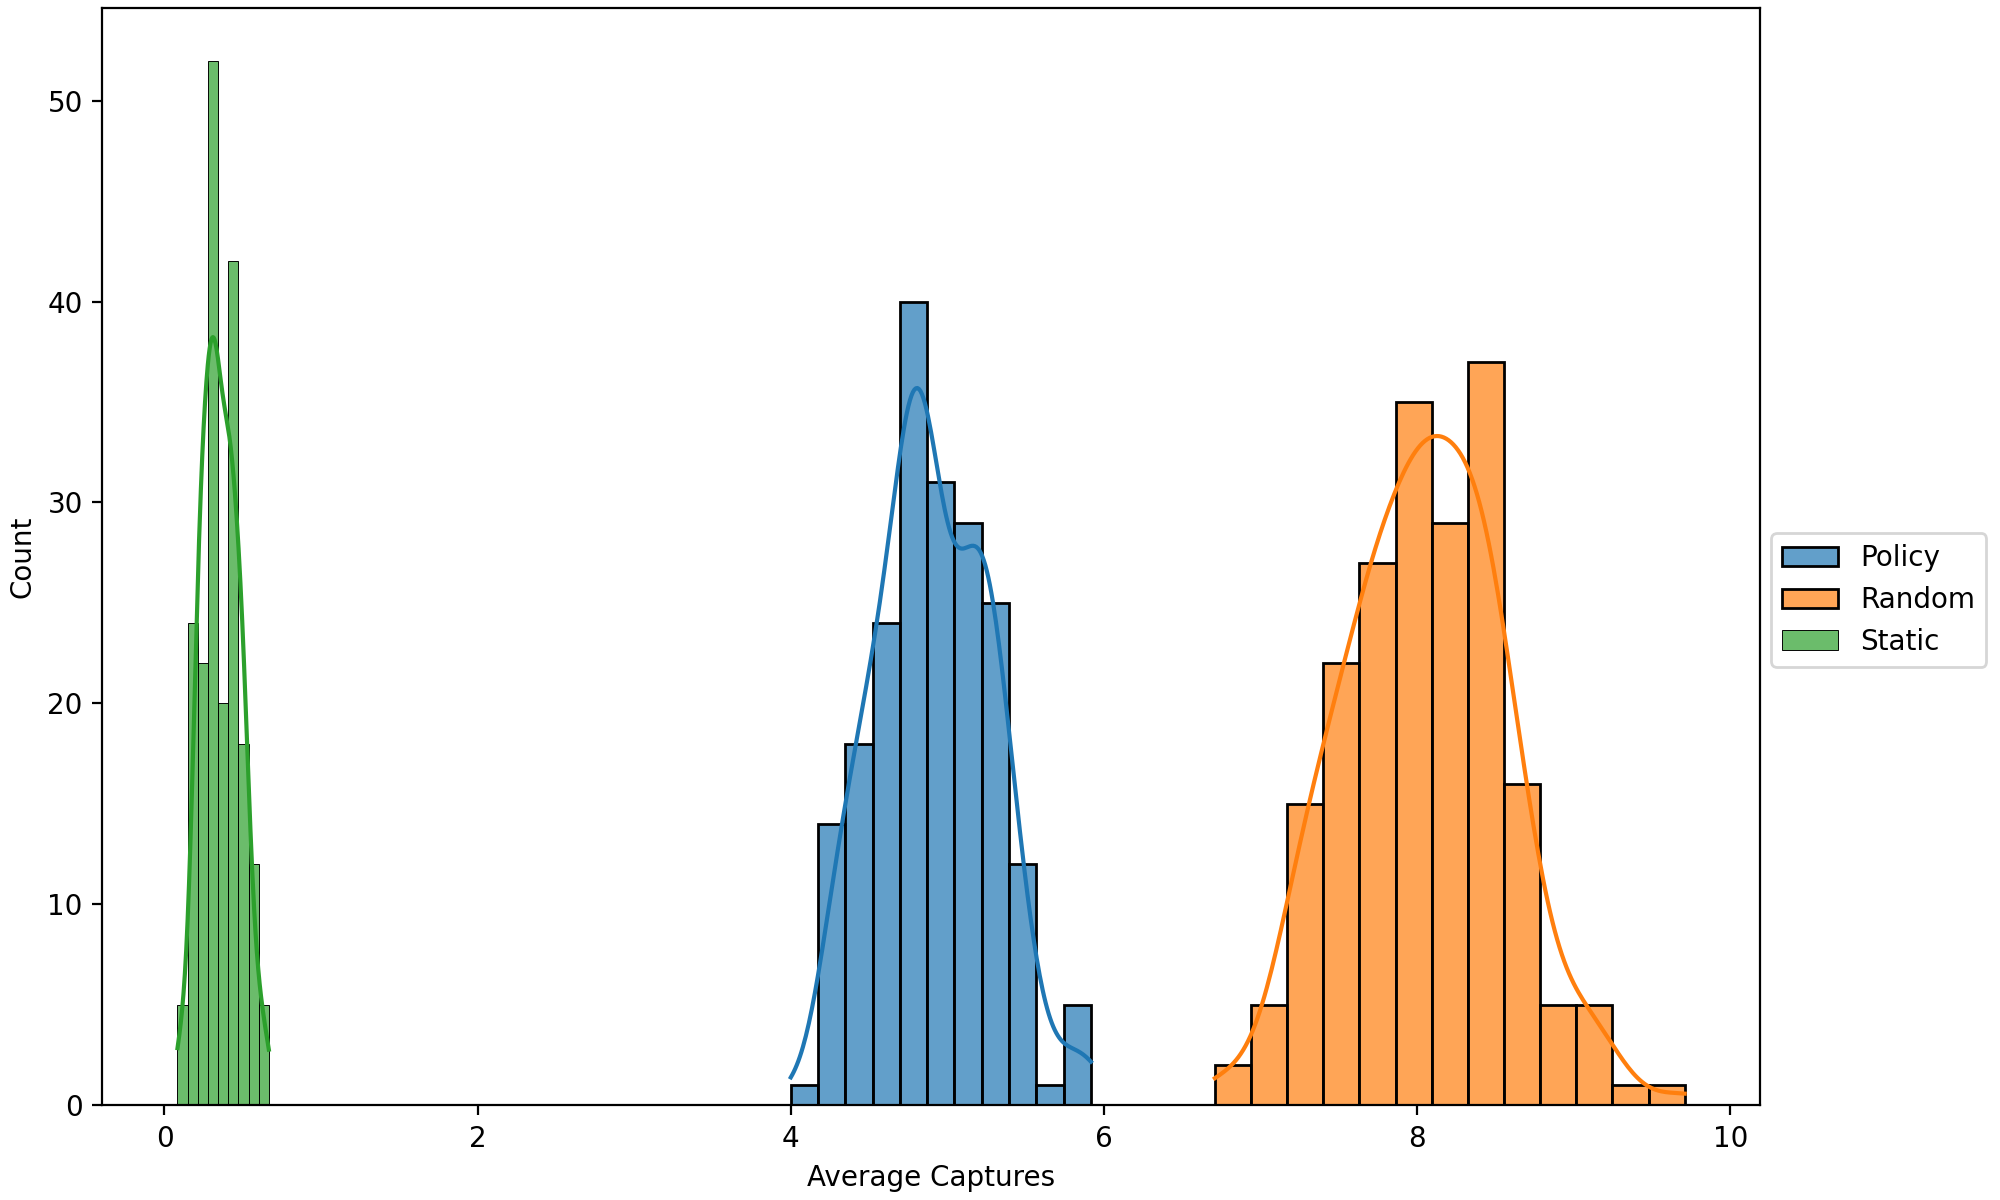}
%      \caption[Distributions of the Average Captures of Three Different Models.]{Distributions of the Average Captures of Three Different Models. The trained policy (individual training, blue), the random model (orange), and the "Turnaway" algorithm (green) were executed across 200 episodes, each consisting of 3000 time steps, using five distinct seeds in an environment featuring a single predator governed by the static "NaivChase" algorithm.}
%     \label{fig:indi_captures_combined}
% \end{figure}
